# Supplementary material for: Relational Visual Similarity
Source: arXiv:2512.07833 source file (2026-04-09)

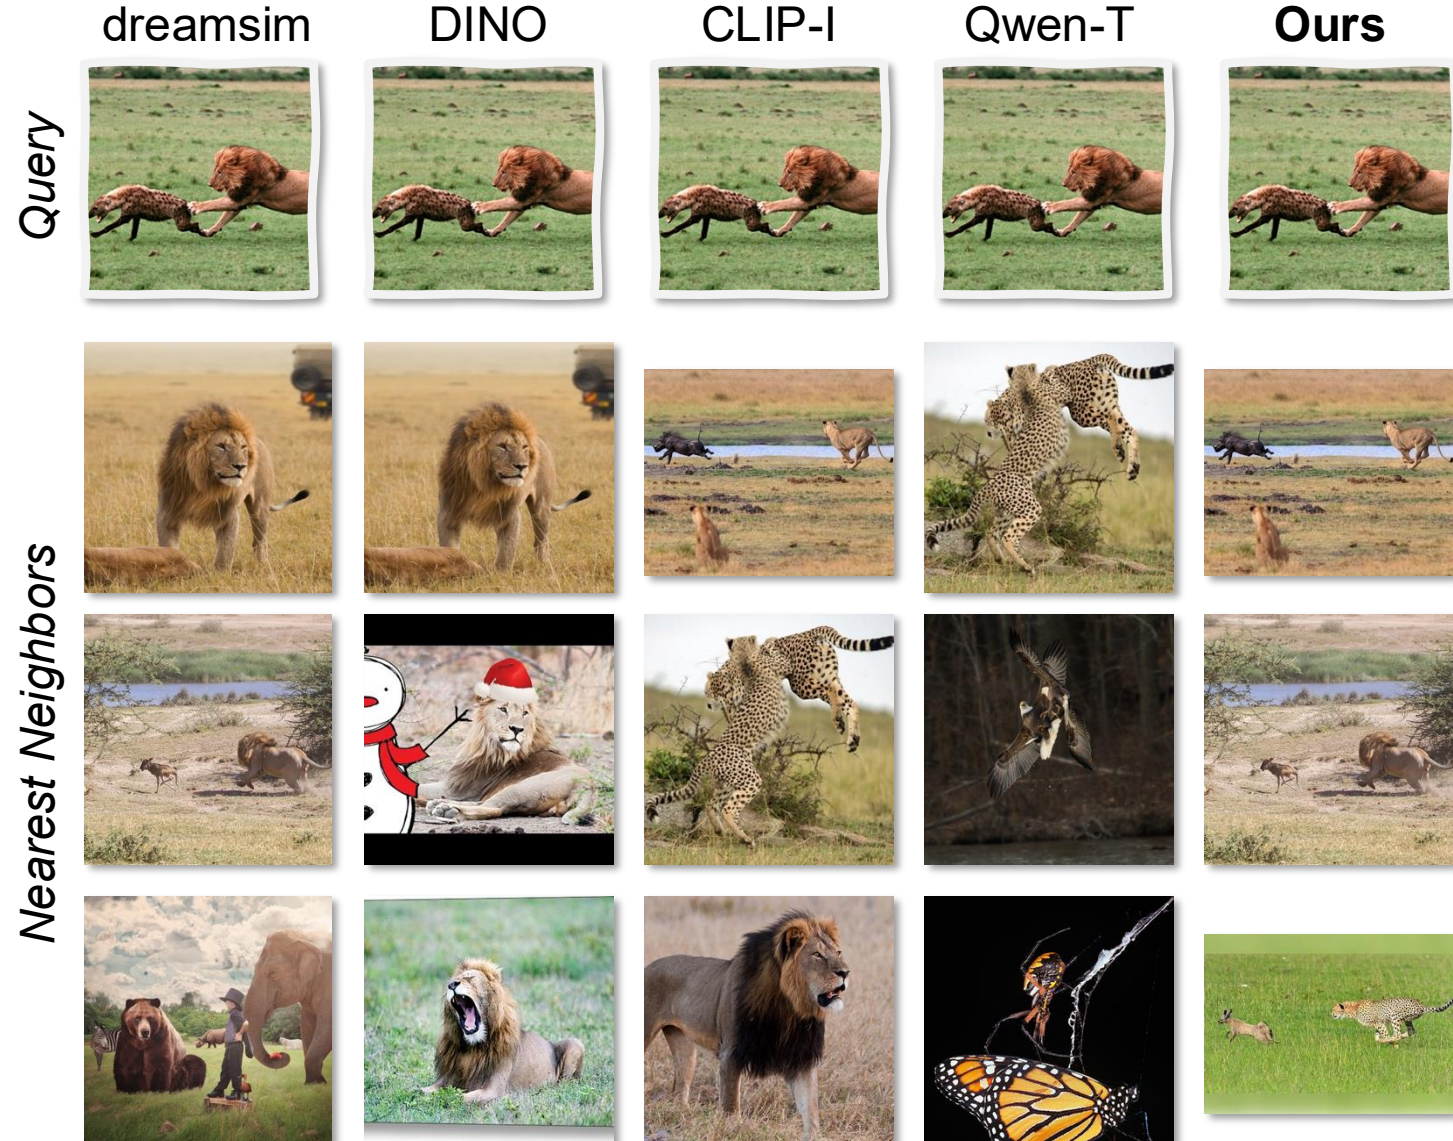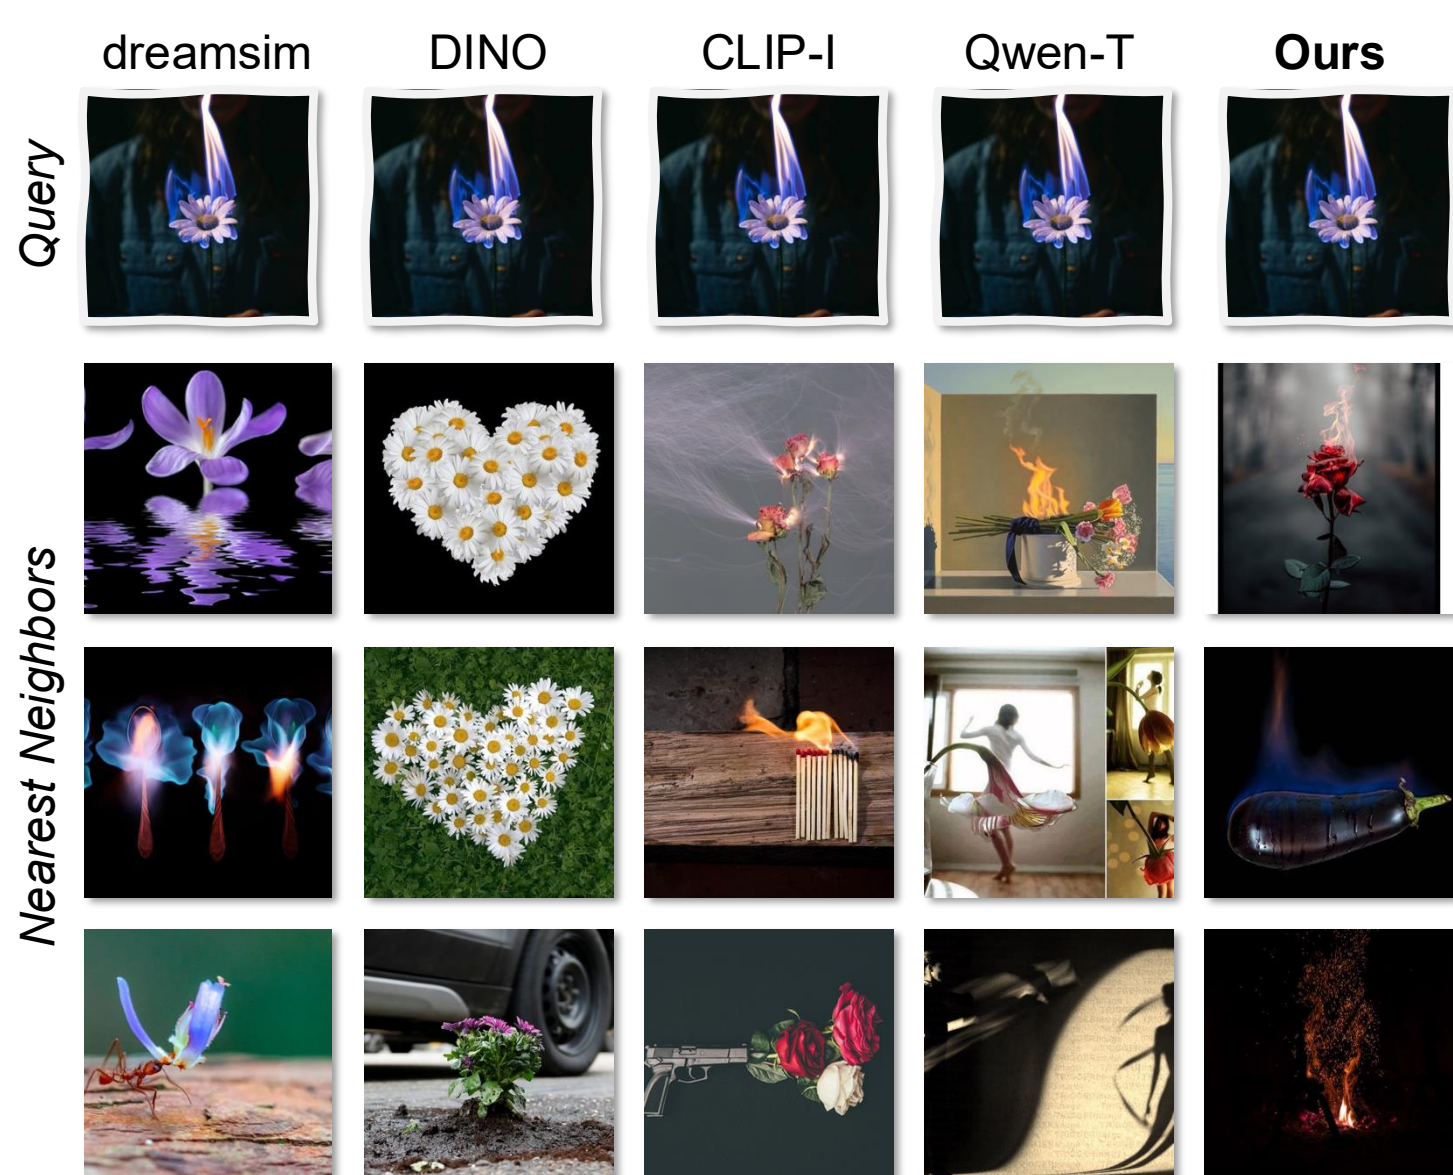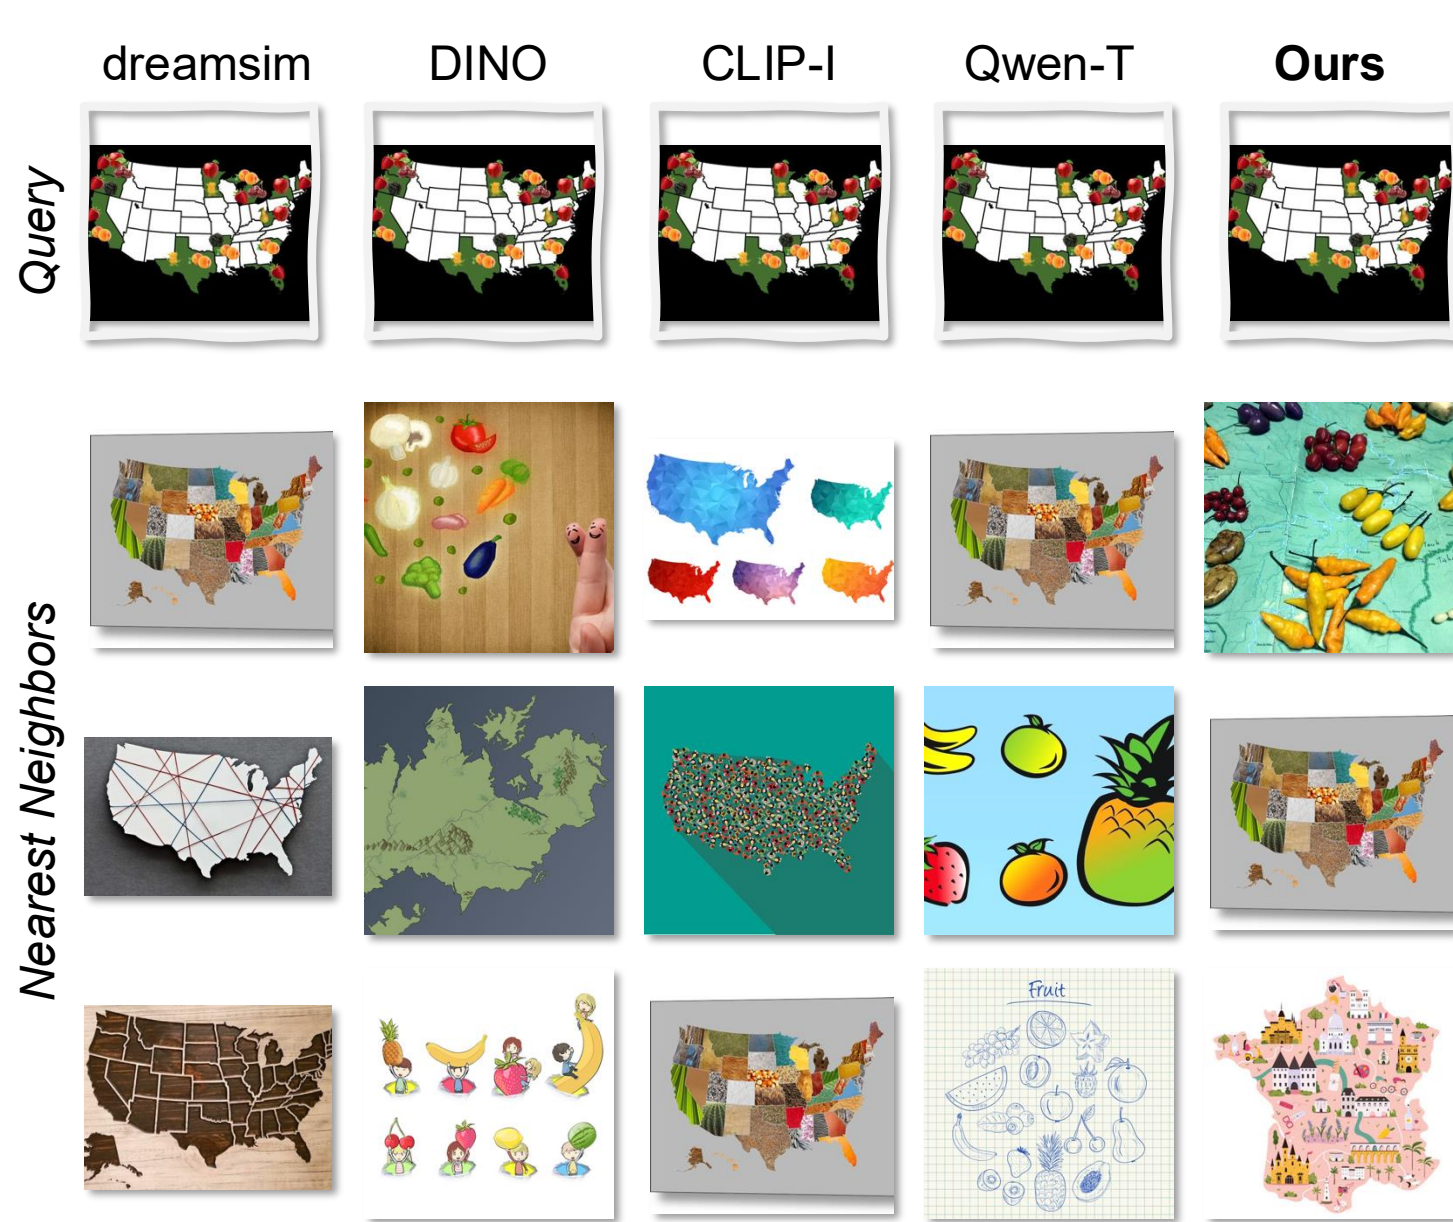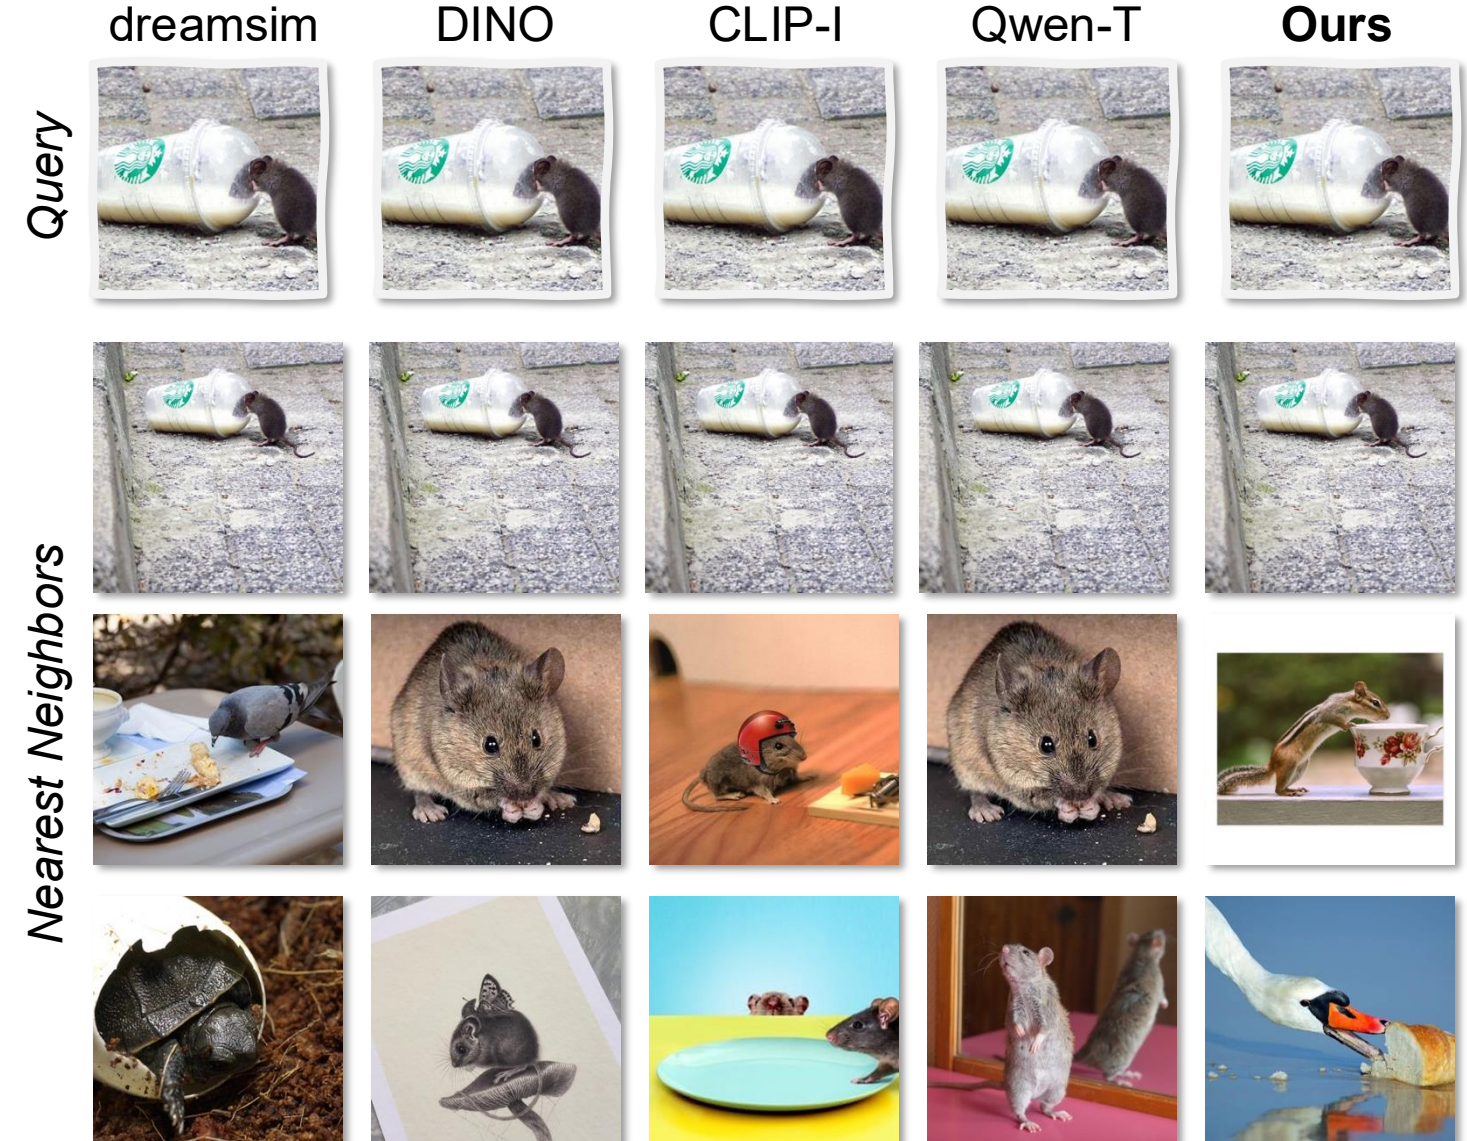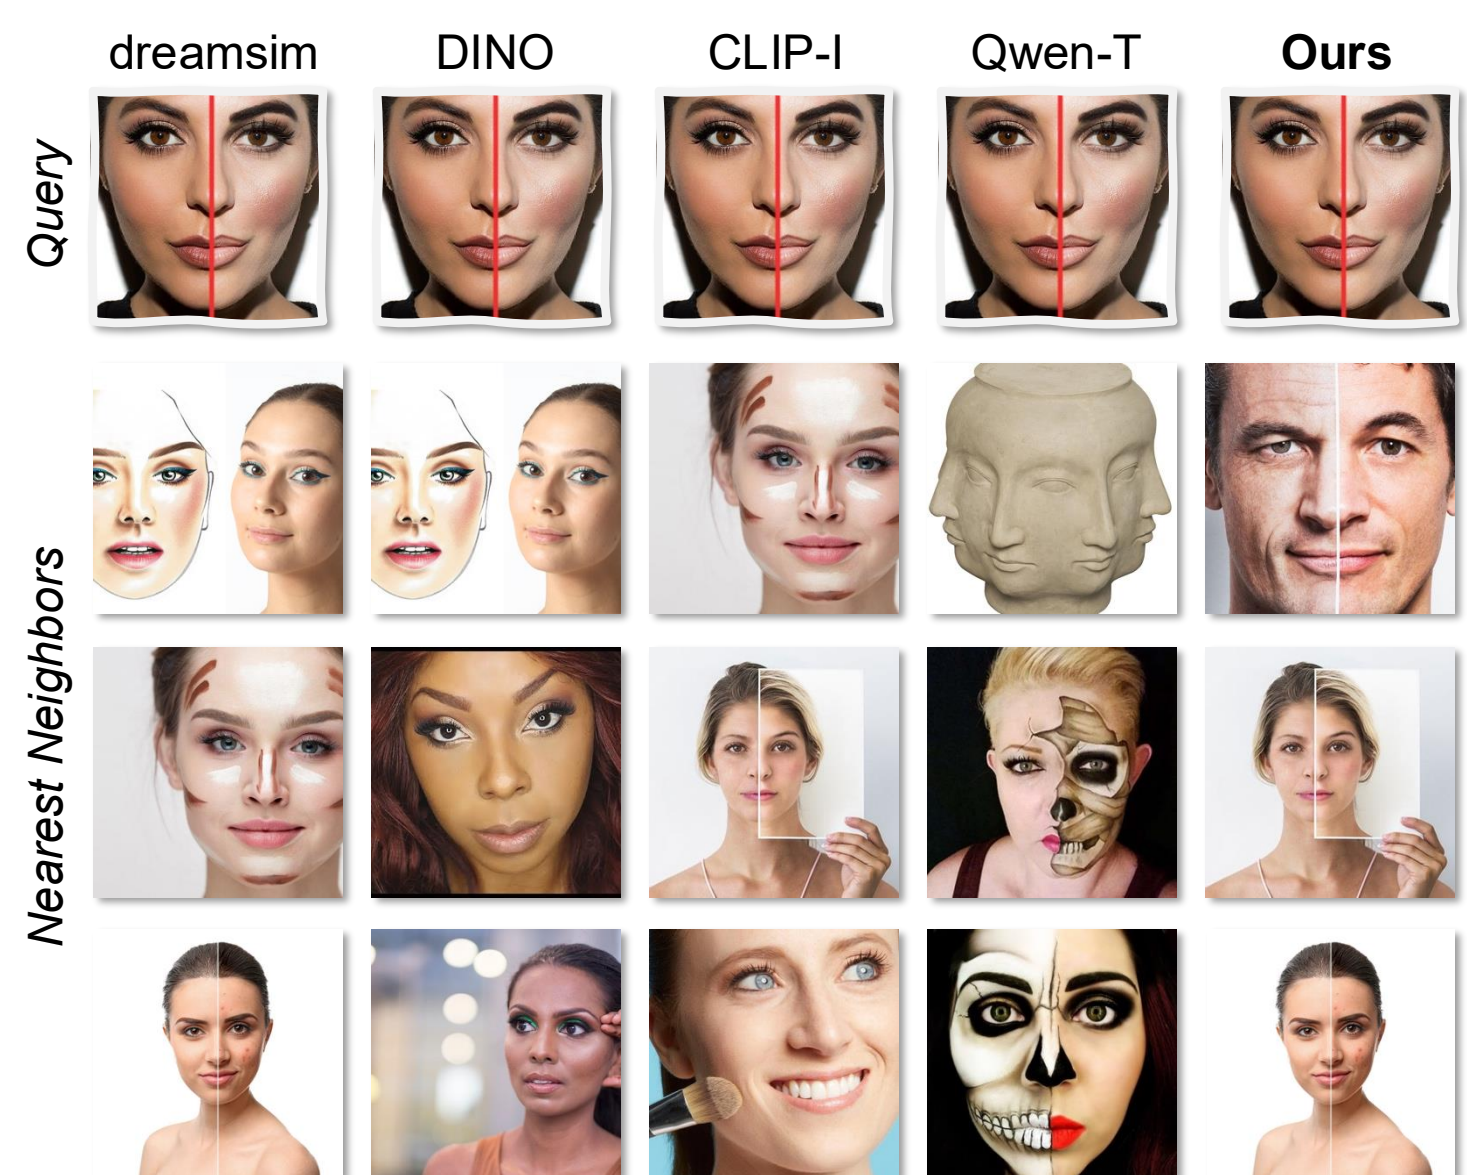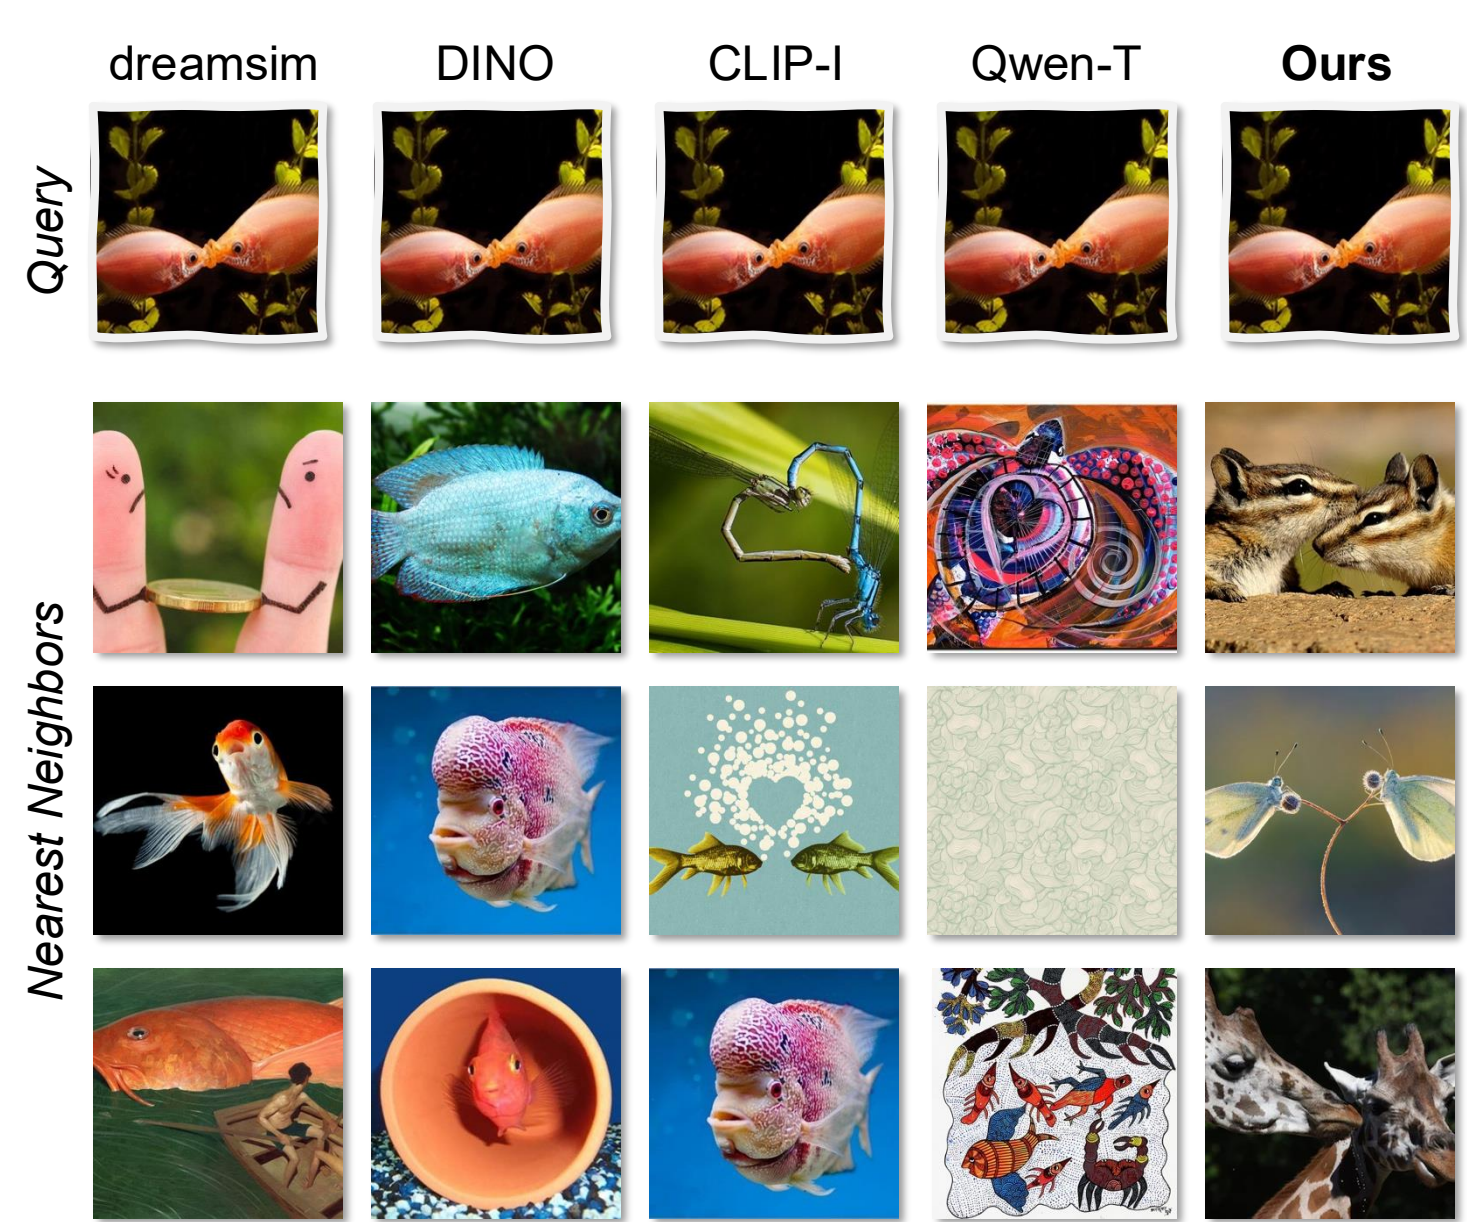



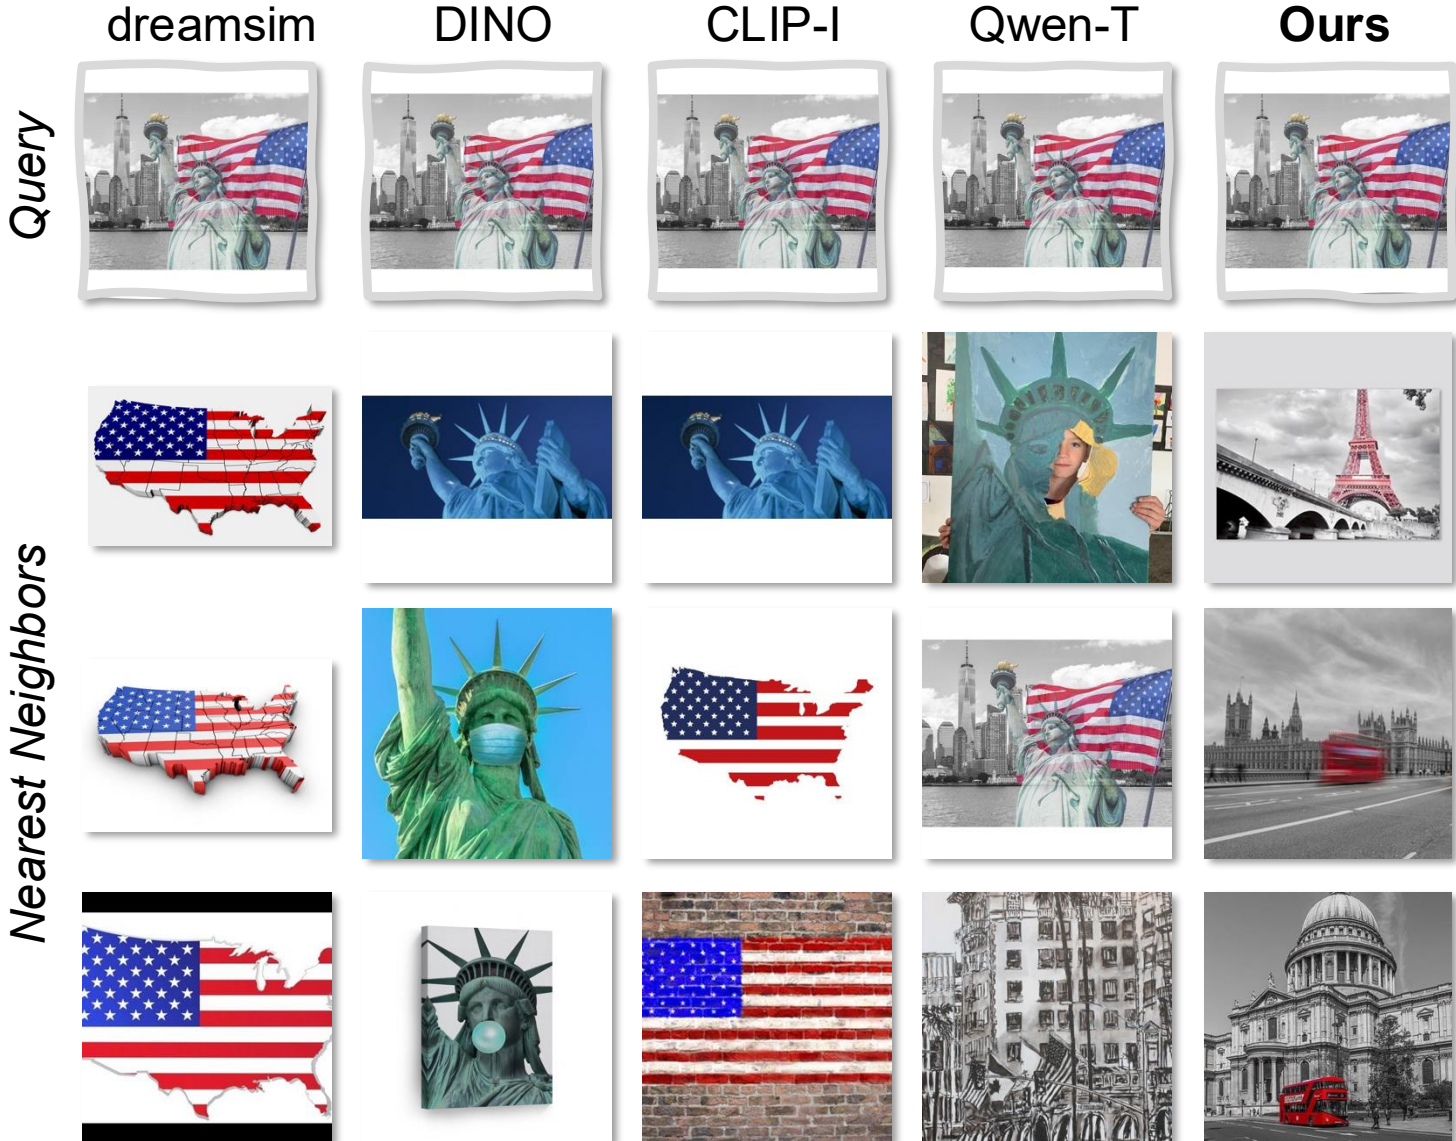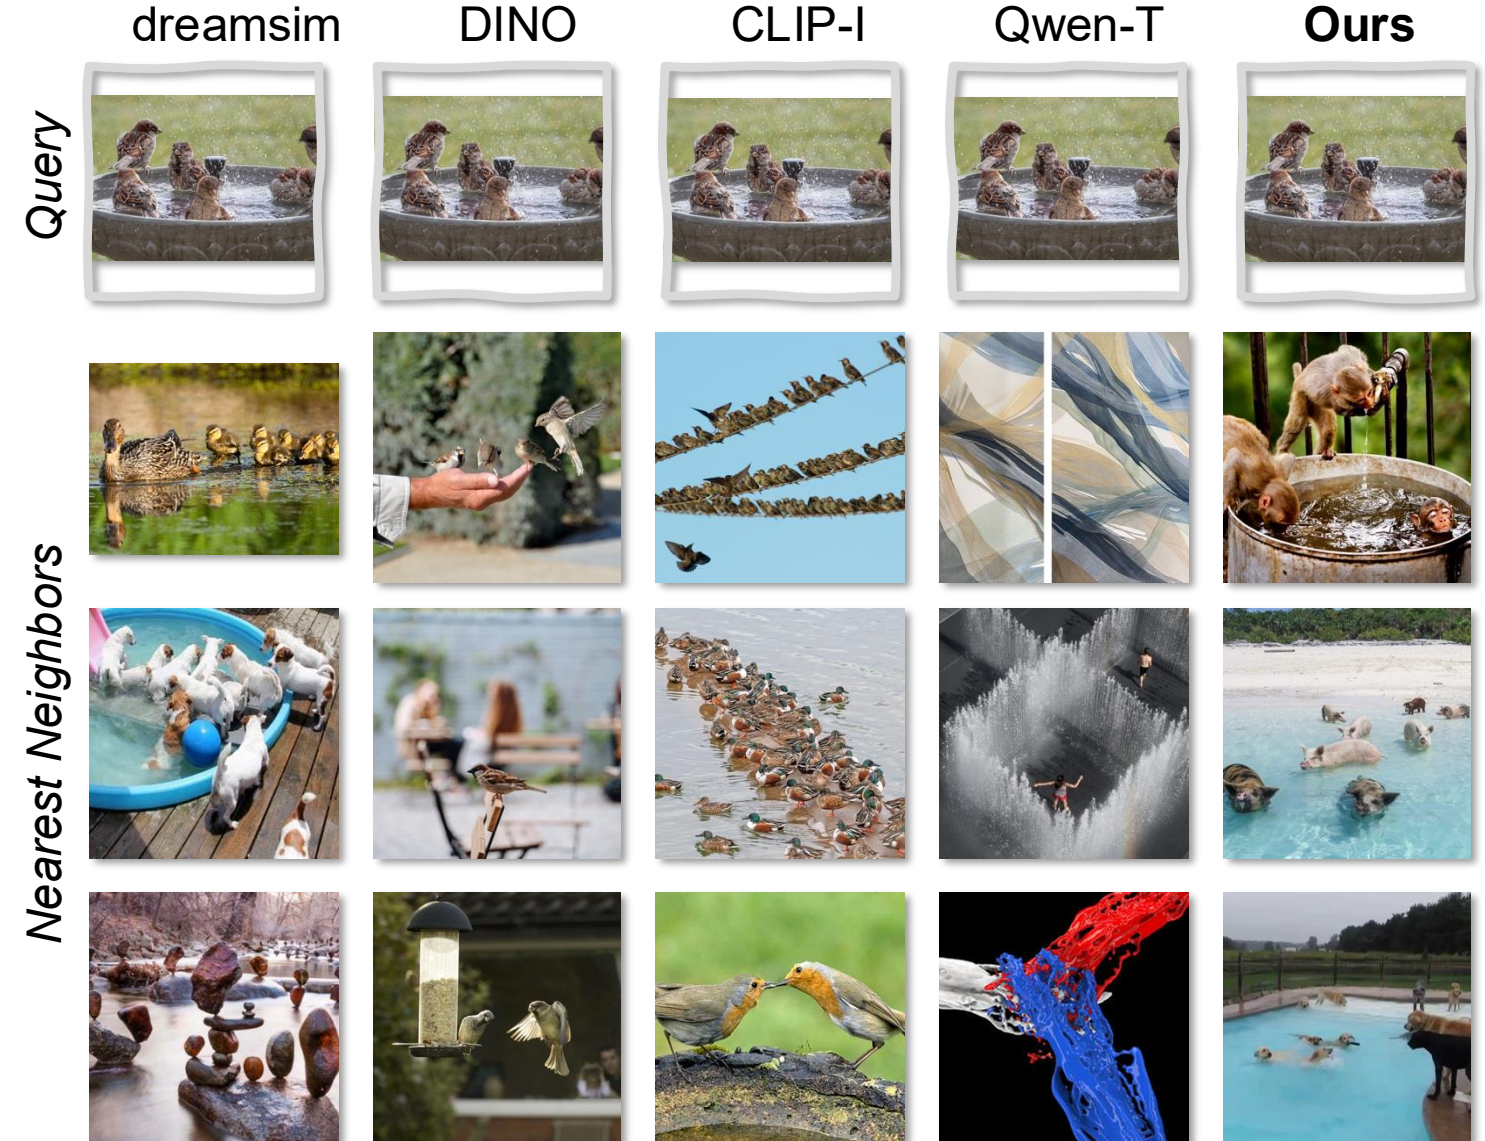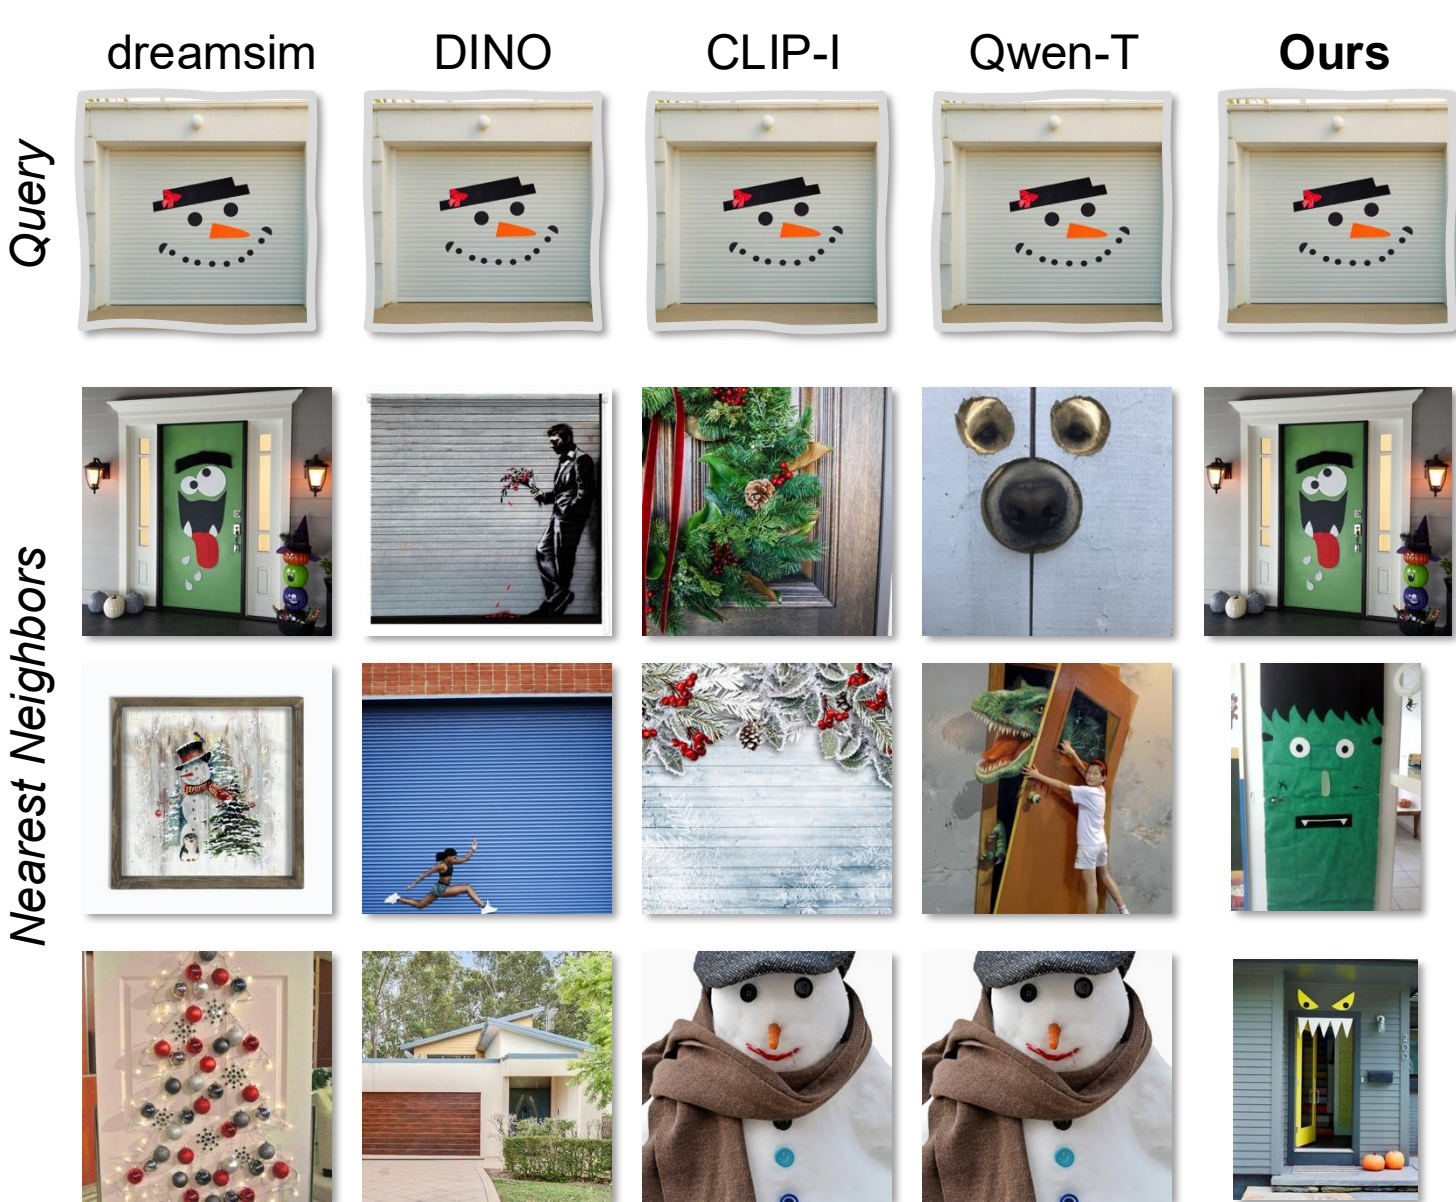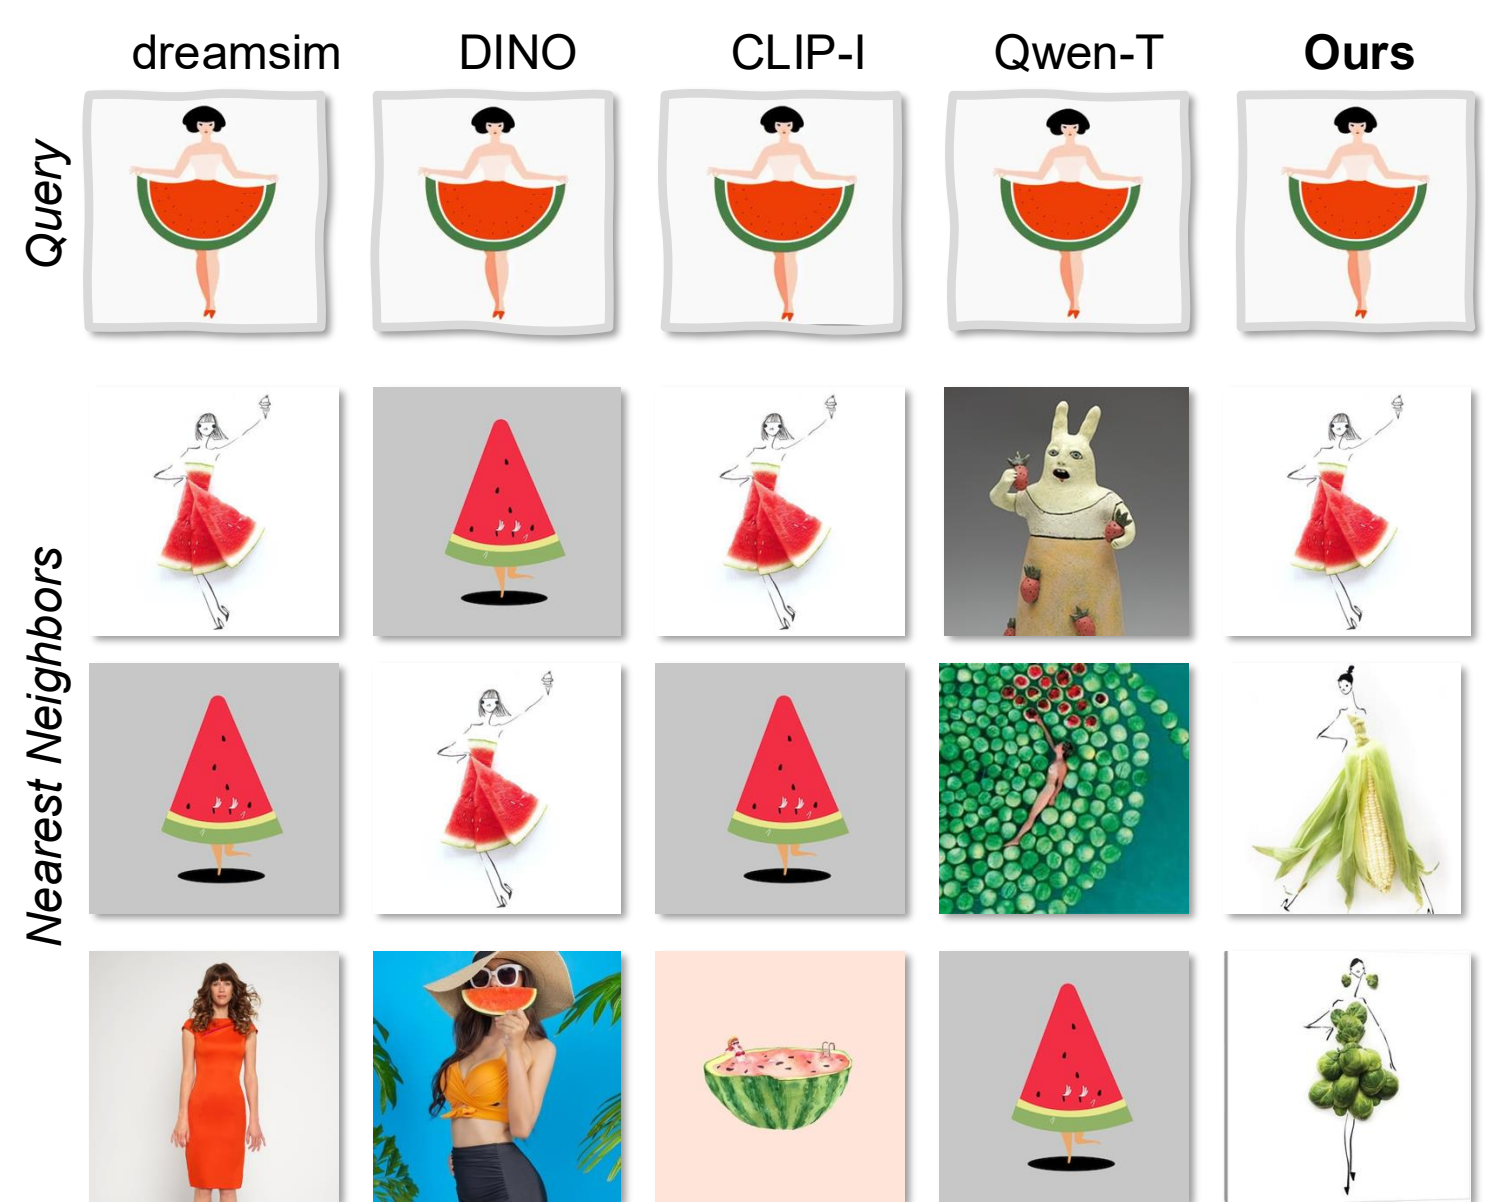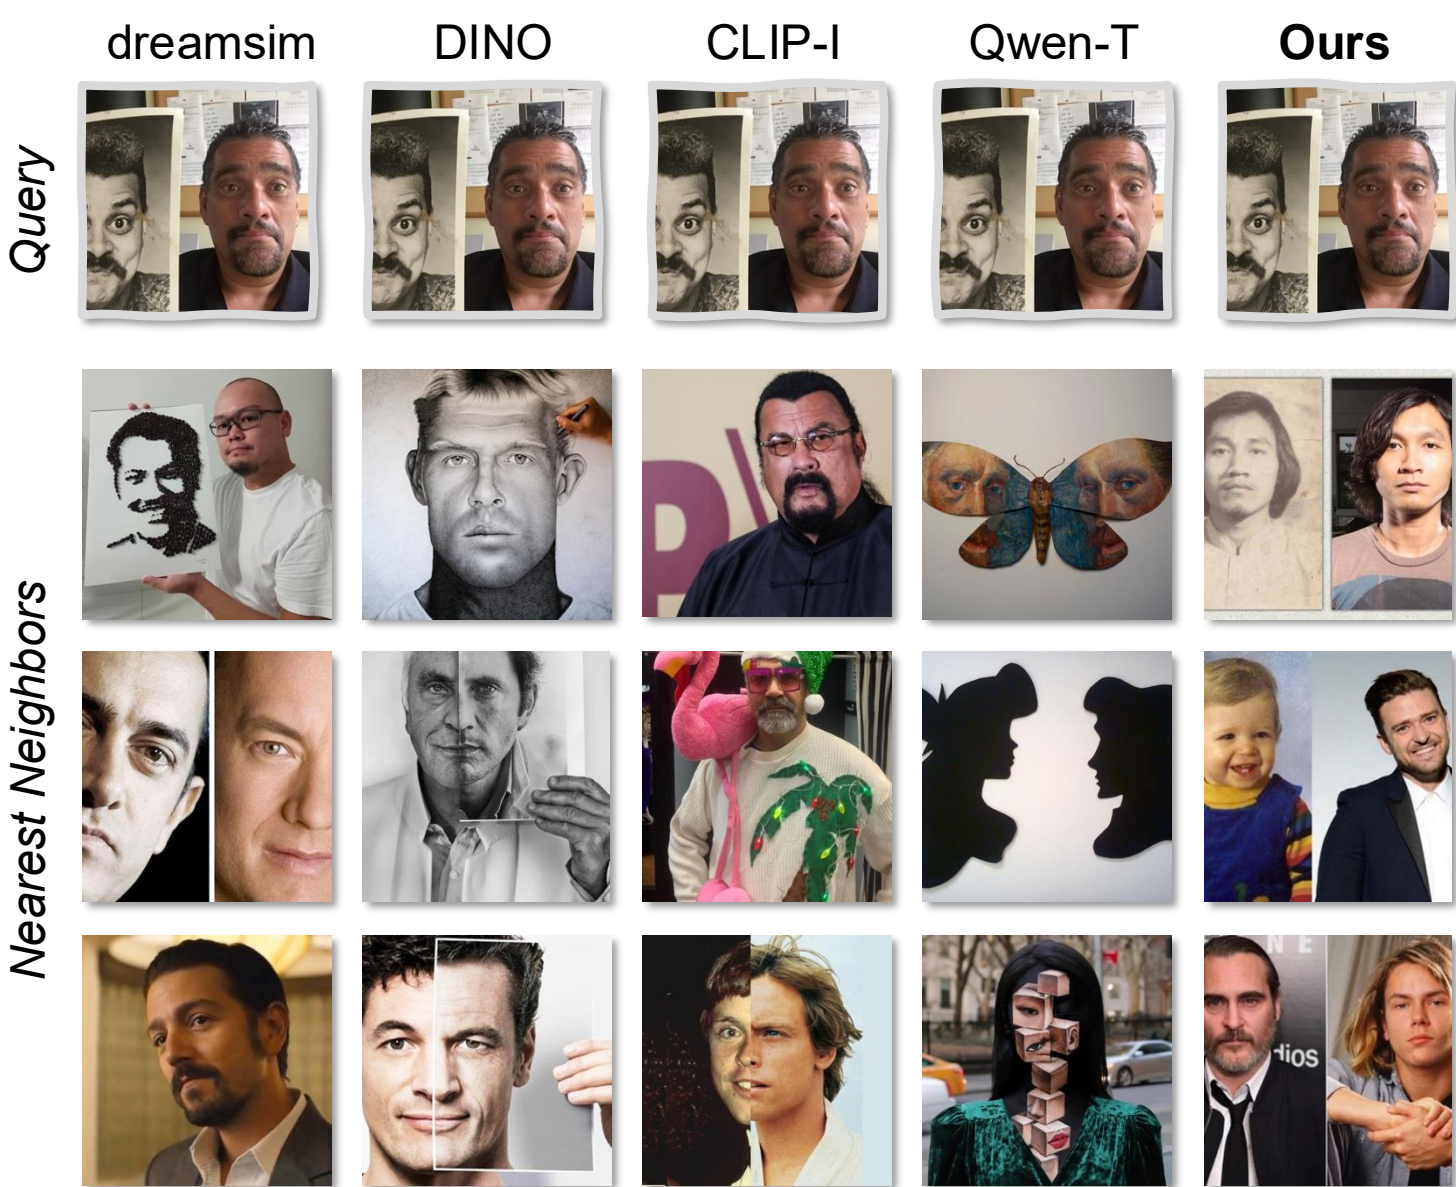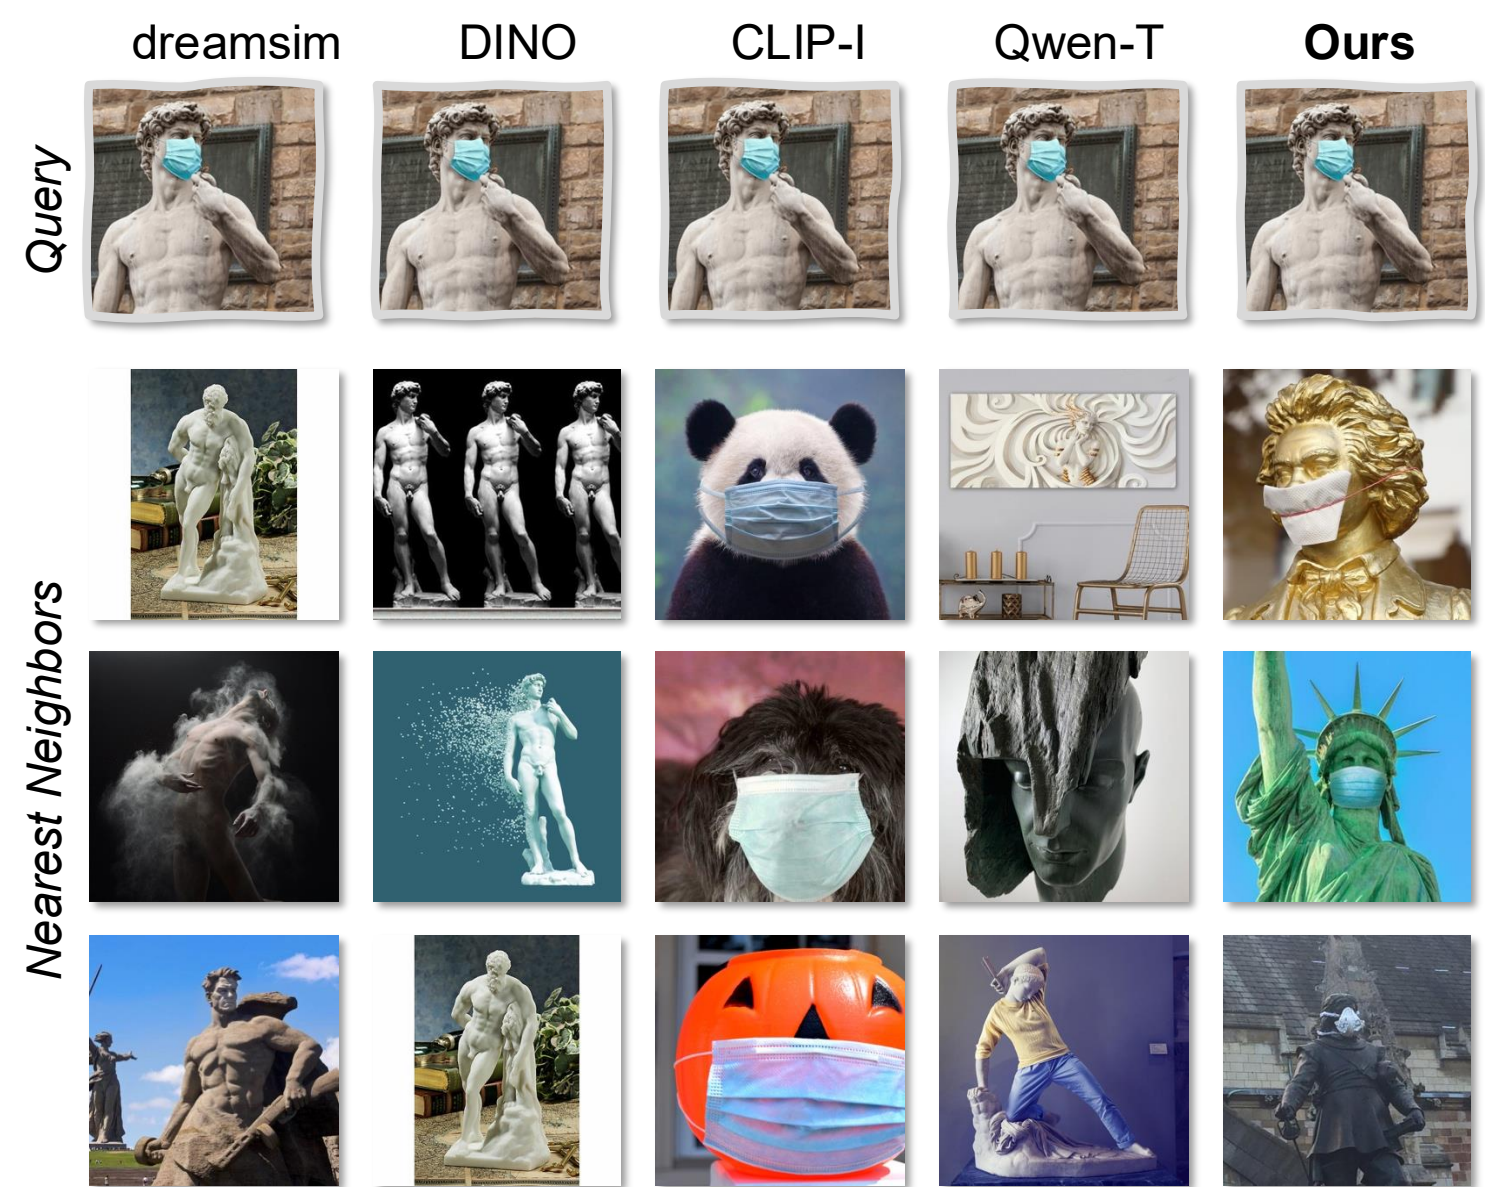

Supplement: Supplementary file 1 [file supp-baselines.pdf]
